# Supplementary material for: Towards high-sensitivity magnetometry with nitrogen vacancy centers in diamond using the singlet infrared absorption
Source: arXiv:2410.20876 source file (2024-10-28)
Supplement: Supplementary file 1 [file SM.pdf]

# Supplemental Materials for

## Towards high-sensitivity magnetometry with nitrogen vacancy centers in diamond using the singlet infrared absorption

Ali Tayefeh Younesi<sup>1</sup>, Muhib Omar<sup>2,3</sup>, Arne Wickenbrock<sup>2,3</sup>, Dmitry Budker<sup>2,3,4</sup>, Ronald Ulbricht<sup>1,\*</sup>

<sup>1</sup>Max Planck Institute for Polymer Research, Ackermannweg 10, 55128 Mainz, Germany

<sup>2</sup>Helmholtz-Institut Mainz, GSI Helmholtzzentrum für Schwerionenforschung GmbH, 55128 Mainz, Germany

<sup>3</sup>Johannes Gutenberg-Universität Mainz, 55128 Mainz, Germany

<sup>4</sup>Department of Physics, University of California, Berkeley, California 94720-300, USA

\* Corresponding author: ulbricht@mpip-mainz.mpg.de

This PDF file includes:

### Contents

|   |                                                  |   |
|---|--------------------------------------------------|---|
| 1 | Ground triplet state ( $^3A_2$ ) in $NV^-$ ..... | 1 |
| 2 | Diamond sample properties and absorption.....    | 2 |
| 3 | Transition rates in $NV^-$ .....                 | 3 |
| 4 | ODMR results using IR absorption.....            | 4 |
| 5 | Microwave (MW) delivery system .....             | 7 |
| 6 | Shot-noise sensitivity calculations.....         | 8 |
| 7 | Sensitivity calculation.....                     | 8 |
| 8 | Calibrating the magnetic field sensor .....      | 9 |

### 1 Ground triplet state ( $^3A_2$ ) in $NV^-$

The ground state of negatively charged nitrogen vacancy ( $NV^-$ ),  $^3A_2$ , is an electronic spin-triplet state with  $m_s = 0, \pm 1$ . The  $m_s = \pm 1$  states are degenerate at zero magnetic field and lie above  $m_s = 0$  with the energy of 2.87 GHz, which is the zero field splitting (ZFS). By applying a magnetic field, the  $m_s = -1$  and  $+1$  energy level split proportional to the applied magnetic field (Zeeman splitting). In this case, the transition frequencies from  $m_s = 0$  to  $m_s = \pm 1$  are given by the following equation

$$\nu_{\pm} = D \pm \frac{g_e \mu_B}{h} B_{NV}$$

where  $D$  is the zero field splitting,  $g_e \approx 2$  is the electronic  $g$  factor,  $\mu_B$  is the Bohr magneton,  $h$  is Planck's constant, and  $B_{NV}$  is the projection of the magnetic field onto the  $NV$  axis.

Beside the Zeeman splitting in the ground state, nuclear spins result in hyperfine splitting. In this case, the energy level of the NV center experience hyperfine splitting due to the nuclear spin of the nitrogen atom, where it can be  $^{14}\text{N}$  or  $^{15}\text{N}$ , which are spin-1 and spin-1/2 systems, respectively. The sample used here is  $^{12}\text{C}$  enriched, which eliminates the  $^{13}\text{C}$  nuclear spin contribution. The nitrogen defects are  $^{14}\text{N}$ , resulting in three states for each electronic spin. The  $^{14}\text{N}$  hyperfine splitting is 2.16 MHz [1] and the resulting splitting in the ground triplet-state of  $\text{NV}^-$  is shown in Figure SM1.

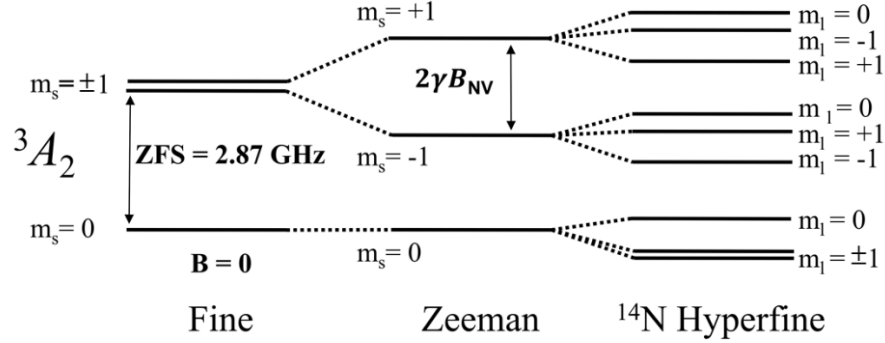

**Figure SM1.** Ground triplet electronic structure of  $\text{NV}^-$  with Zeeman splitting and  $^{14}\text{N}$  hyperfine structure due to nitrogen nuclear spin.  $\gamma = \frac{2g_e\mu_B}{h}$  is the gyromagnetic ratio for the NV center.

Within  $\text{NV}^-$  center's pump cycle, the electrons in  $m_s = 0$  in the excited triplet state ( $^3E$ ) mostly relax to  $m_s = 0$  in  $^3A_2$  by PL, whereas electrons with  $m_s = \pm 1$  are more likely to have an inter-system crossing (ISC) than  $m_s = 0$ , thus establishing optical spin polarization. By photo-exciting  $\text{NV}^-$  centers, after a few pump cycles, the ground spin-triplet ( $^3A_2$ ) is polarized and most of the electrons are in the  $m_s = 0$  state. Furthermore, the ZFS of 2.87 GHz between  $m_s = 0$  and  $\pm 1$  in  $^3A_2$ , enables the opportunity to drive the spin state in the ground state between  $m_s = 0$  and  $\pm 1$  by applying a microwave (MW) signal.

## 2 Diamond sample properties and absorption

The sample is a  $^{12}\text{C}$  enriched CVD grown bulk diamond (Element Six). The nitrogen concentration of the sample before NV creation is 13 ppm. The NV concentration including both charge states is around 4 ppm. The absorption of the sample with a thickness of 0.5 mm is shown in Figure SM1.

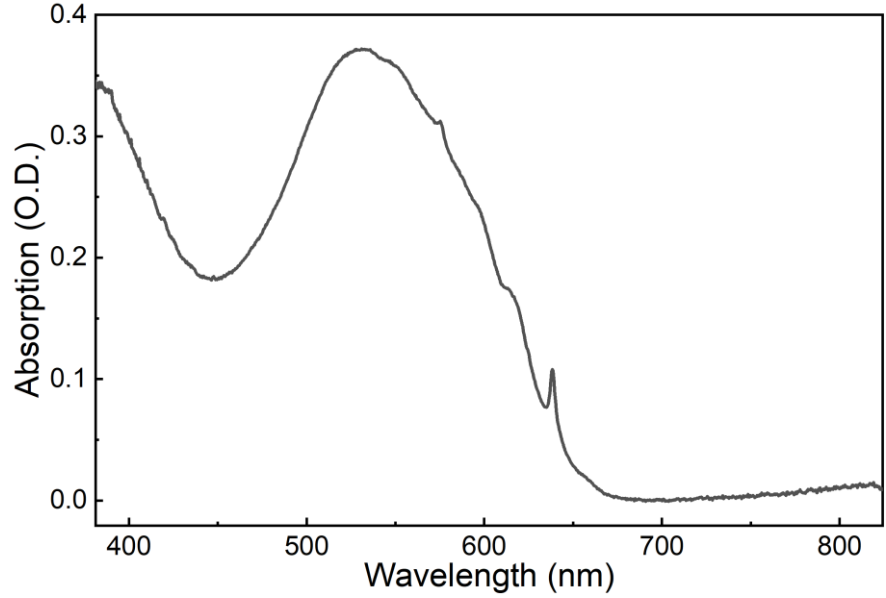

**Figure SM 2.** The absorption spectrum of the sample. The zero-phonon line (ZPL) of  $\text{NV}^-$  at 637 nm and its phonon-sideband (PSB) on the blue side is visible. Some amount of neutrally charged NV ( $\text{NV}^0$ ) can also be identified, recognizable by the ZPL peak at 575 nm.

### 3 Transition rates in $\text{NV}^-$

As shown in the schematic of  $\text{NV}^-$  in Fig. 1-a (reproduced for convenience as Figure SM 3), by pumping the sample, the excited electrons have two relaxation paths. They either relax down to the ground triplet-state by photoluminescence (PL), or by the non-radiative channel through the singlet states ( ${}^3E \rightarrow {}^1A_1 \rightarrow {}^1E \rightarrow {}^3A_2$ ) via intersystem crossings (ISC). The ratio of PL and ISC is spin selective. Electrons with spin  $m_s = \pm 1$  tend to have higher probability of having an ISC than the  $m_s = 0$  state [2]. Due to the transition rates of these states (as stated in Fig. 1-a), the lower singlet state,  ${}^1E$ , remain populated for longer time after pumping in comparison with other state, creating an additional absorption zero-phonon line at 1042 nm (1.19 eV). Because of the nature of spin-selective ISC, this IR absorption can be used to readout the electron spin in the ground triplet state.

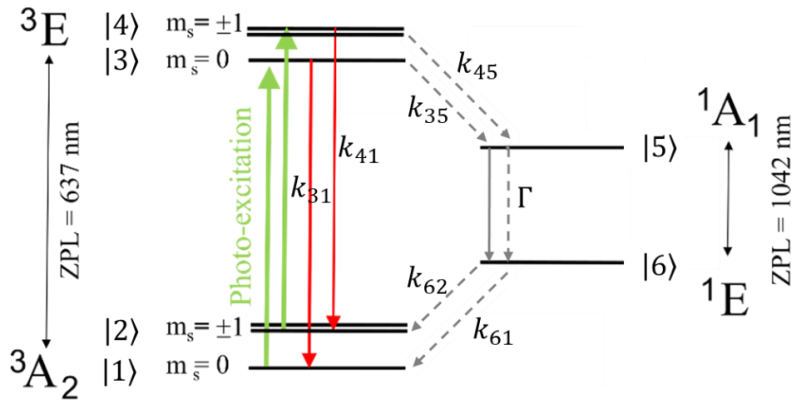

**Figure SM 3.** Schematic of  $\text{NV}^-$  with the transition rates shown on each arrow  $k_{ij}$ .

In order to quantify the spin contrast, the transition rates for the six-level system NV that is sketched in Figure SM 3, is listed in the Table 1. Given the parameters in the table, the spin selectivity of ISC and PL is noticeable i.e. different rates for ISC and PL from  $m_s = 0$  and  $m_s = \pm 1$ . By comparing their values, it can be concluded that the ISC-involved process (i.e. IR transition) has higher spin contrast due to higher spin selectivity in the ISC path. The spin selectivity for PL detection from  $m_s = 0$  is calculated to be  $\sim 44\%$ , while for the ISC-involved process (i.e. IR transition) from  $m_s = \pm 1$ , it is approximately 89%. These values are calculated on the assumption of equal electron population in all  $m_s = 0$  and  $\pm 1$  of the excited state  ${}^3E$ , followed by the relaxation with the rates listed below.

| PARAMETER                      | RATE VALUE                |
|--------------------------------|---------------------------|
| $k_{31} = k_{42}$ (PL)         | $(66 \pm 5)\mu s^{-1}$    |
| $k_{35}$ (ISC <sub>1</sub> )   | $(7.9 \pm 4.1)\mu s^{-1}$ |
| $k_{45}$ (ISC <sub>1</sub> )   | $(53 \pm 7)\mu s^{-1}$    |
| $k_{61}$ (ISC <sub>2</sub> )   | $(1.0 \pm 0.8)\mu s^{-1}$ |
| $k_{62}$ (ISC <sub>2</sub> )   | $(0.7 \pm 0.5)\mu s^{-1}$ |
| $\Gamma$ (non-radiative decay) | $10\text{ ns}^{-1}$       |

Table 1. Transition rates of the six-level system sketched in Figure SM 3. The rates  $k_{ij}$  are obtained from [3] and  $\Gamma$  is measured in [4].

#### 4 ODMR results using IR absorption

As described before, by measuring the IR absorption and manipulating the electron spin, we can readout the spin states of the electrons. Here, a microwave (MW) signal is scanned around the zero-field splitting (ZFS) and the transmitted IR beam is measured. Because of the four possible orientations of NV in the crystal, each of them may have different projection of the applied magnetic field along their axes. The ODMR plot in a case that the applied magnetic field has different projection on each NV axis is shown in Figure SM 4, black curve. In this case, the different projection causes different Zeeman splitting for each NV orientation. Each splitting also has three peaks due to hyperfine splitting of  ${}^{14}N$ . Because of the preferred polarization dependent of the optical beams and the MW source, two peaks have higher intensity than the other two.

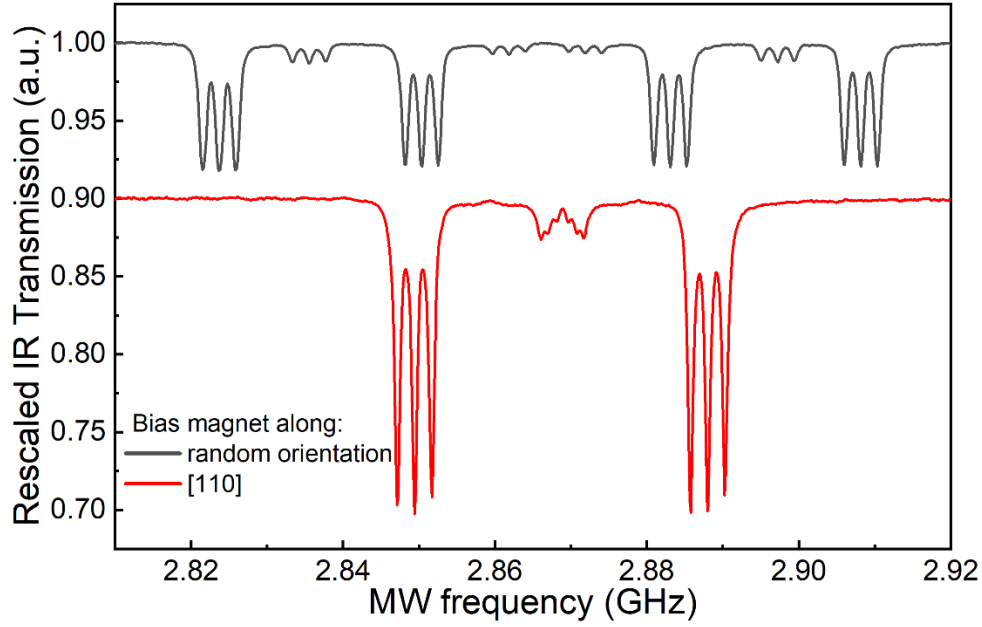

**Figure SM 4.** The ODMR graph when a bias magnetic field is applied at a random orientation creating different magnetic field projections on each NV axis (black curve) and when it is applied along [110], creating two pairs of peaks (red curve). The DC level of the red curve is shifted for better illustration.

By aligning the applied magnetic field along [110] orientation, the projection of the magnetic field on two NV axes ( $[111]$  and  $[\bar{1}\bar{1}1]$ ) are equal and the angle between them is  $35.3^\circ$ , and the angle with the other two axes ( $[1\bar{1}\bar{1}]$  and  $[\bar{1}11]$ ) is  $90^\circ$ . This bias field orientation creates two pairs of overlapping NV axes, shown in Figure SM 4, red curve. The graph with four peaks is fitted with six Lorentzian function and the fitting is shown Fig. 3-a, upper window (in the manuscript), and the fitting parameters are listed in the Table 2. The contrast is the intensity of the ODMR peak for a single hyperfine splitting in the normalized IR transmission graph.

| Peak Index | FWHM (MHz) | Contrast (%) | Central frequency (MHz) |
|------------|------------|--------------|-------------------------|
| 1          | 0.85       | -0.54        | 2851.23                 |
| 2          | 0.82       | -0.53        | 2853.39                 |
| 3          | 0.80       | -0.52        | 2855.53                 |
| 4          | 0.83       | -0.58        | 2885.32                 |
| 5          | 0.84       | -0.55        | 2887.46                 |
| 6          | 0.84       | -0.54        | 2889.61                 |

**Table 2.** The fitting parameters of the CW ODMR graph shown in Fig. 3-a with six Lorentzian functions.

The ODMR plot is measured for various MW powers and the ratio of the contrast and FWHM is calculated to find the optimum MW power. The calculated parameters for a single peak are plotted in Figure SM 5. The x-axis is the MW power that is applied to the input of the MW amplifier (with a gain of 46 dB).

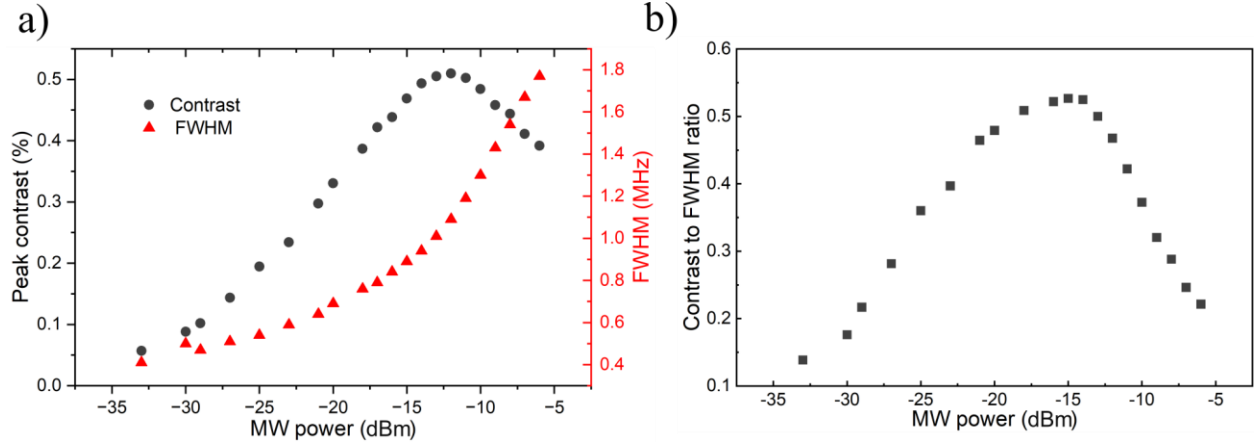

**Figure SM 5.** CW ODMR peak contrast and FWHM for peak number 2 (listed in Table 2) for various MW powers.

Driving the hyperfine transitions at the same time increases the contrast to FWHM ratio, thus the magnetic sensitivity. Besides, addressing both transitions for  $m_s = 0 \leftrightarrow m_s = -1$ , and  $m_s = 0 \leftrightarrow m_s = +1$  further increases the ratio. Therefore, with the MW mixing technique, we drive all hyperfine transitions for NV oriented along  $[111]$  and  $[\bar{1}\bar{1}1]$ . In this case, the ODMR plot has five peaks shown in Fig. 3-b in the manuscript. It is fitted with five Lorentzian peaks with the parameters listed in Table 3.

| Peak Index | FWHM (MHz) | Contrast (%) | Central frequency (MHz) |
|------------|------------|--------------|-------------------------|
| 1          | 0.55       | -0.67        | -4.32                   |
| 2          | 0.65       | -1.2         | -2.16                   |
| 3          | 0.70       | -1.6         | 0.01                    |
| 4          | 0.67       | -1.19        | 2.18                    |
| 5          | 0.57       | -0.65        | 4.35                    |

Table 3. Fitting parameters of the CW ODMR when exciting all hyperfine splitting, which creates five peaks, shown in Fig. 3-b.

In this case, the MW power is scanned to find the optimum power. The contrast, FWHM and their ratio is plotted in Figure SM 6. The x-axis is the power of the MW signal generator that is then mixed with the output of the other signal generator (SG2, shown in Fig. 1-c) using a mixer. The MW power before the MW amplifier is measured using an oscilloscope, and for 8 dBm input power, it results in -22 dBm for each peak intensity. Total power at the input of the MW amplifier is -14 dBm.

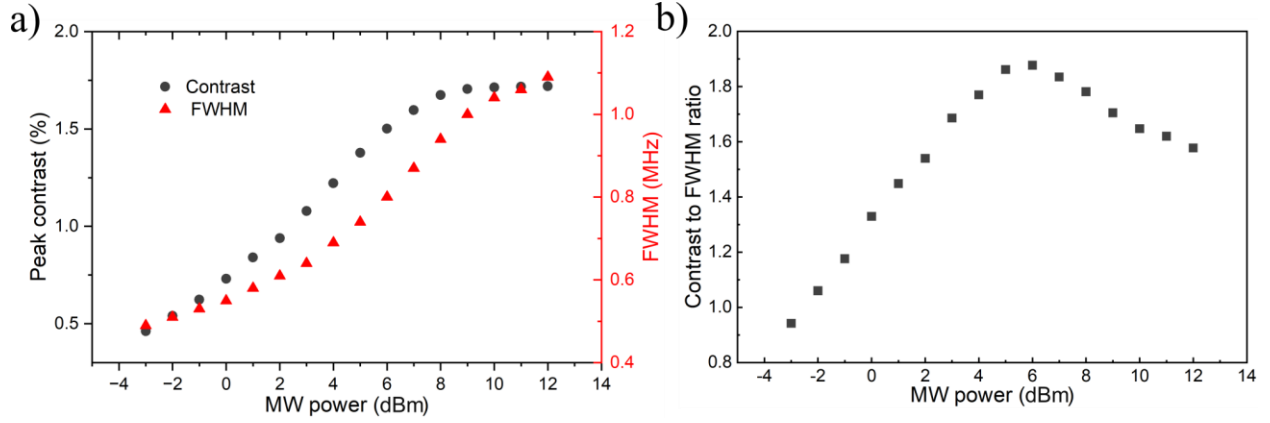

**Figure SM 6.** The CW ODMR peak contrast and FWHM for peak number 3 (listed in Table 3) for various MW powers. This is the case when all the hyperfine levels for both  $m_s = \pm 1$  are excited by the MW signal.

## 5 Microwave (MW) delivery system

As briefly mentioned in the manuscript, a radio frequency (RF) system is implemented to generate the desired MW signal. This includes a MW signal generator SG1, SG396 Stanford Research Systems, a custom sine wave generator, SG2 (a homemade VHDL code to run on the FPGA board of Moku:Pro, Liquid Instruments), an RF mixer (ZX05-U4324H-S+, Mini-Circuits), an RF amplifier (ZHL-15W-422X-S+, Mini-Circuits), and a circulator terminated with a 50 Ohm resistance (UIYBCC6434A2T4SF, UIY). To drive all hyperfine transitions, SG1 generates a sine wave at central frequency of the zero-field splitting (ZFS),  $f_{SG1} = f_{ZFS} = 2.87$  GHz. SG2 generates three sine waves with central frequency  $f_c$  and sidebands at  $f_c \pm 2.16$  MHz.  $f_c$  is adjusted to be equal to the Zeeman splitting of the  $m_s = \pm 1$  states,  $f_c = g_e \mu_B B_{NV}$  and 2.16 MHz is the hyperfine splitting energy due to  $^{14}\text{N}$ . The output of SG1 is connected to local oscillator (LO) of the mixer and the SG2 output is connected to intermediate frequency pin (IF). The output of the mixer is given by the following equation.

$$S_{Applied} = \sin(2\pi(f_{ZFS} + f_c)t) + \sin(2\pi(f_{ZFS} + f_c + 2.16 \text{ MHz})t) \\ + \sin(2\pi(f_{ZFS} + f_c - 2.16 \text{ MHz})t) + \sin(2\pi(f_{ZFS} - f_c)t) \\ + \sin(2\pi(f_{ZFS} - f_c - 2.16 \text{ MHz})t) + \sin(2\pi(f_{ZFS} - f_c + 2.16 \text{ MHz})t)$$

This signal is then connected to the RF amplifier whose output is connected to a circulator. The output of the circulator is connected to a closed wire loop on the sample. The applied MW signal to the amplifier is measured using an oscilloscope and plotted in Figure SM 7.

For the magnetometry measurement, the frequency of SG2 output is modulated with a modulation frequency of  $f_{mod} = 5.6$  kHz and deviation amplitude of  $f_{dev} = 330$  kHz. In this case, the input signal of the amplifier is given by the following equation.

$$S_{Applied} = \sin(2\pi(f_{ZFS} + f_c)t + f_{dev} \sin 2\pi f_{mod} t) \\ + \sin(2\pi(f_{ZFS} + f_c + 2.16 \text{ MHz})t + f_{dev} \sin(2\pi f_{mod} t)) \\ + \sin(2\pi(f_{ZFS} + f_c - 2.16 \text{ MHz})t + f_{dev} \sin(2\pi f_{mod} t)) \\ + \sin(2\pi(f_{ZFS} - f_c)t - f_{dev} \sin(2\pi f_{mod} t)) \\ + \sin(2\pi(f_{ZFS} - f_c - 2.16 \text{ MHz})t - f_{dev} \sin(2\pi f_{mod} t)) \\ + \sin(2\pi(f_{ZFS} - f_c + 2.16 \text{ MHz})t - f_{dev} \sin(2\pi f_{mod} t))$$

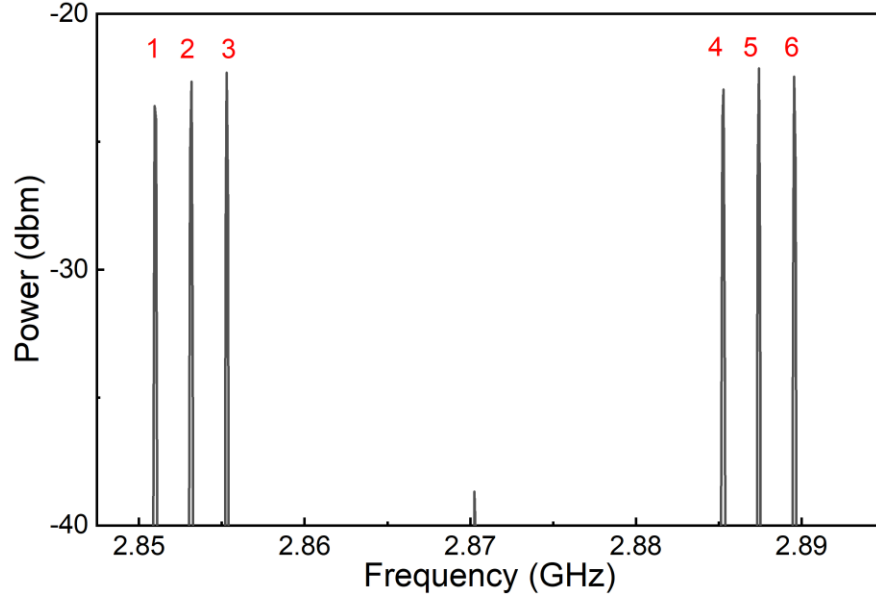

**Figure SM 7.** The power spectrum of the applied MW signal to the amplifier at 6 frequencies addressing all hyperfine states for both  $m_s = \pm 1$ .

## 6 Shot-noise sensitivity calculations

To calculate the shot-noise sensitivity for CW ODMR, we use

$$\eta_{CW} = \frac{4}{3\sqrt{3}} \frac{h}{g_e \mu_B} \frac{\Delta\nu}{C_{CW} \sqrt{R}}$$

where  $h$  is Planck's constant,  $g_e$  is NV electronic g factor,  $\mu_B$  is the Bohr magneton,  $\Delta\nu$  and  $C_{CW}$  are the linewidth and the contrast of the ODMR peak, respectively, and  $R$  is the photon-detection rate [6]. In our measurements, by driving all the hyperfine splitting transitions simultaneously for  $m_s = 0 \leftrightarrow m_s = -1$  and  $m_s = 0 \leftrightarrow m_s = +1$ , a contrast of,  $C_{CW}$ , 1.6% and linewidth,  $\Delta\nu$ , 0.7 MHz are achieved. Here,  $R$  is calculated from the power of the detected IR on the photodiode, which is around 12 mW. These parameters result in an estimated shot-noise sensitivity of around

$$\eta_{CW} \approx 5 \frac{\text{pT}}{\sqrt{\text{Hz}}}.$$

Given the sensitivity noise floor mentioned in the manuscript (18 pT/ $\sqrt{\text{Hz}}$ ), further sensitivity improvements are possible. Furthermore, using this technique, since the shot-noise limit is determined by the external IR light source power, it can be further reduced by increasing the IR power.

## 7 Sensitivity calculation

In order to calculate the sensitivity graph, the LIA output that is demodulated at the  $f_{mod}$  of the MW signal, is first recorded for 60 seconds and is converted to the magnetic field with the conversion ratio. Then, the data is split to 60 1-second long measurements and the power spectral density for each 1-second segment is calculated using the Fourier transform and by taking the square root of that the linear spectral density is determined. Finally, all of the spectral density curves are averaged together, which gives the sensitivity graph. The reason of splitting the data into 1-second segments is because the linear spectral density (LSD) might have a different value than the linear spectrum (LS) which gives the root square mean (rms) and their ratio is given by:

$$LSD = \frac{LS}{\sqrt{ENBW}}$$

where ENBW is effective noise bandwidth and is given by:

$$ENBW = NENBW \cdot \frac{f_s}{N}$$

and NENBW is the normalized equivalent noise bandwidth,  $f_s$  is the sampling frequency, and N is the number of data points [7]. The NENBW depends on the window function used in calculating the Fourier transform and for a rectangular window, its value is 1. Given the equations, if  $f_s = N$ , the linear spectral density is equal to linear spectrum. Therefore, the measured magnetic field LSD has the same value as the rms value of the applied field at the specified frequency.

## 8 Calibrating the magnetic field sensor

As described in the manuscript, the output of the lock-in amplifier (LIA) is proportional to the magnetic field with the following equation

$$\Delta B_{NV} = S_{LIA} \frac{h}{g_e \mu_B \alpha \cos \theta}$$

where  $\theta$  is the angle between the measured magnetic field and NV axis ( $35.3^\circ$ ), and  $\alpha$  is proportional to  $C_{CW}/\Delta\nu$ . In order to calculate  $\alpha$ , the central frequency of the applied MW is shifted by a known value, then the change in the LIA output is measured. Then, by knowing the other physical constants, the LIA output is converted to magnetic field intensity.

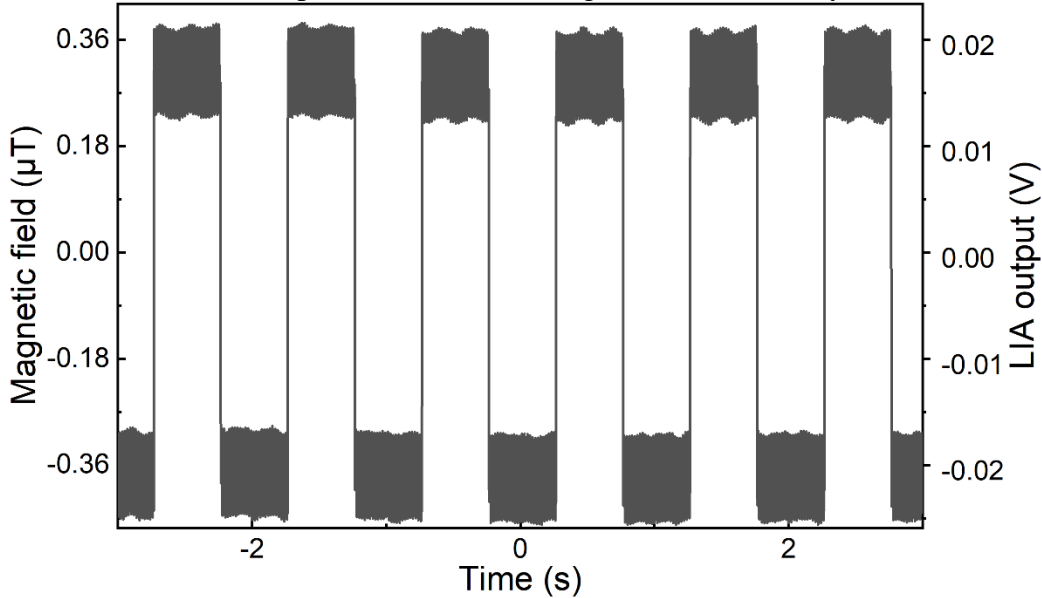

**Figure SM 8.** Applied test field with peak-peak intensity of 0.71  $\mu\text{T}$  with a frequency of 1 Hz measured with the sensor and the output voltage of the LIA is plotted.

In order to make sure that the measured magnetic field is correct, we also perform a test measurement with a known magnetic field. The magnetic field is applied by a homemade coil with a radius of  $r = 20$  mm,  $N = 10$  turns, and placed at a distance about  $d = 26$  mm from the sample. The coil is connected to a signal generator in series with a 1 k $\Omega$  resistor. The generated magnetic field by the coil is given by:

$$B_{rms} = \frac{\mu_0 I_{rms} N}{2} \frac{r^2}{(r^2 + d^2)^{3/2}}$$

where  $I_{rms}$  is given by the rms applied voltage ( $V_{rms}$ ) divided by the 1 k $\Omega$  resistance in series. First, a 10 V peak-peak voltage is applied to the coil at frequency of 1 Hz. The LIA output is plotted in Figure SM 8. The calculated applied magnetic field from the equation mentioned above is 0.71  $\mu$ T, and the measured parameter (shown in Figure SM 8), is 0.69  $\mu$ T, which is within 3% error bar.

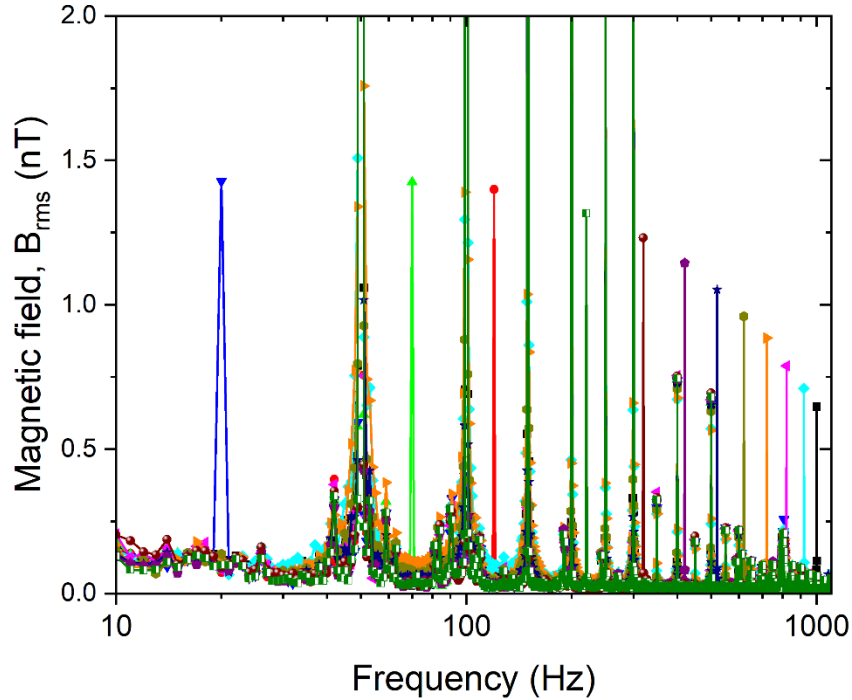

**Figure SM 9.** Magnetic field spectrum when test magnetic fields are applied at various frequencies. The peaks at 50 Hz and its higher harmonics are due to the line power magnetic noise in the laboratory.

For further testing the magnetic sensor, AC magnetic fields at different frequencies are applied to the sample in the frequency range is from 20 to 1000 Hz, which is illustrated in Figure SM 9. The measured values for multiple frequencies are listed in Table 4. As shown, the measured value decreases as the frequency increases. The magnetic field intensity calculated by the coil equation is 1.40 nT (20 mV<sub>rms</sub> applied to the coil). Therefore, a calibration factor is required for the sensor to operate at various frequencies. The calibration factor is shown in Figure SM 10. The measured value with the sensor must be multiplied with the calibration factor to calculate the applied magnetic field. This frequency dependent behavior is believed to be due to integration time constant of the lock-in amplifier.

| Frequency (Hz) | Measured $B_{rms}$ (nT) |
|----------------|-------------------------|
| 20             | 1.42                    |
| 70             | 1.42                    |
| 120            | 1.40                    |
| 220            | 1.31                    |
| 320            | 1.23                    |
| 420            | 1.14                    |
| 520            | 1.05                    |
| 620            | 0.96                    |
| 720            | 0.88                    |
| 820            | 0.79                    |
| 920            | 0.71                    |
| 1000           | 0.65                    |

**Table 4.** Measured test magnetic field value at various frequencies.

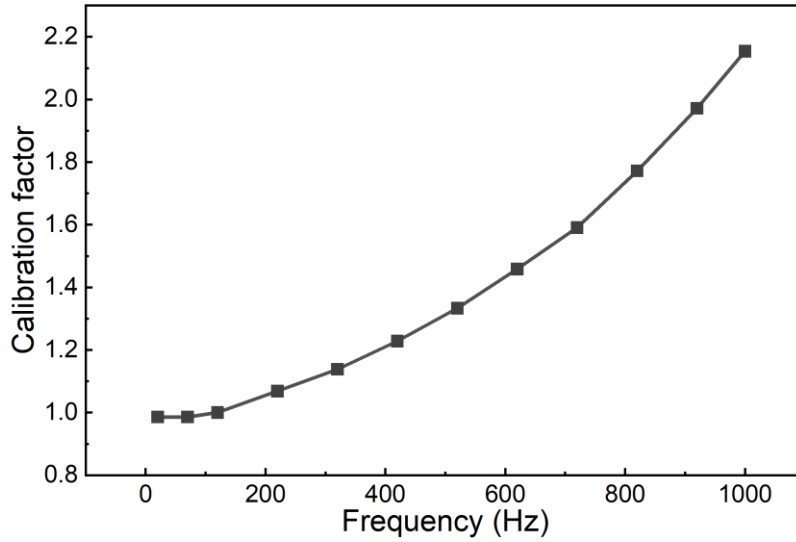

**Figure SM 10.** Calibration factor calculated based on the test magnetic field to calibrate the real applied magnetic field value.

## Acknowledgments

We acknowledge Marc-Jan van Zadel and Florian Gericke for technical support. We acknowledge funding by the Max-Planck Society. We also acknowledge support from the European Commission's Horizon Europe Framework Program under the Research and Innovation Action MUQUABIS GA no. 101070546, by the German DFG, Project SFB 1552 "Defekte und Defektkontrolle in weicher Materie" and funding by the Carl-Zeiss-Stiftung (HYMMS P2022-03-044), also the German Federal Ministry of Education and Research (BMBF) within the Quantumtechnologien program through the DIAQNOS project (project no. 13N16455).

1. Felton, S., et al., *Hyperfine interaction in the ground state of the negatively charged nitrogen vacancy center in diamond*. Physical Review B, 2009. **79**(7): p. 075203.
2. Doherty, M.W., et al., *The nitrogen-vacancy colour centre in diamond*. Physics Reports, 2013. **528**(1): p. 1-45.
3. Dumeige, Y., et al., *Magnetometry with nitrogen-vacancy ensembles in diamond based on infrared absorption in a doubly resonant optical cavity*. Physical Review B, 2013. **87**(15): p. 155202.
4. Ulbricht, R. and Z.-H. Loh, *Excited-state lifetime of the  $N V^-$  infrared transition in diamond*. Physical Review B, 2018. **98**(9): p. 094309.
5. Younesi, A.T. and R. Ulbricht, *Broadband transient absorption spectroscopy using an incoherent white-light source as probe*. Optics Express, 2022. **30**(21): p. 38896-38906.
6. Barry, J.F., et al., *Sensitivity optimization for NV-diamond magnetometry*. Reviews of Modern Physics, 2020. **92**(1): p. 015004.
7. Heinzel, G., A. Rüdiger, and R. Schilling, *Spectrum and spectral density estimation by the Discrete Fourier transform (DFT), including a comprehensive list of window functions and some new at-top windows*. 2002.
